# Supplementary material for: BigMac: Breaking the Pareto Frontier of Compute and Memory in Multimodal LLM Training
Source: arXiv:2605.25451 source file (2026-07-07)
Supplement: Supplementary file 1 [file appendix.tex]

\appendix
\section{Appendix}
\label{appendix}

This is appendix.
